# Supplementary material for: RBF-Solver: A Multistep Sampler for Diffusion Probabilistic Models via Radial Basis Functions
Source: arXiv:2603.13330 source file (2026-03-05)
Supplement: Supplementary file 1 [file main.tex]

\subsection{Comparison with AMED-Solver and AMED-Plugin}

\input{Appendix/calibration/amed/edm_cifar10}
\input{Appendix/calibration/amed/edm_ffhq}
